# Supplementary material for: Learning to Fuse Things and Stuff
Source: arXiv:1812.01192 source file (2019-05-16)
Supplement: Supplementary file 1 [file supplementary.tex]

\begin{table}[]
\centering
\resizebox{0.4\textwidth}{!}{%
\begin{tabular}{@{}lccc@{}}
\toprule
\textbf{Class} & \textbf{PQ} & \textbf{SQ} & \textbf{RQ} \\ \midrule
animal--bird & 0.0 & 0.0 & 0.0 \\
animal--ground-animal & 39.1 & 80.5 & 48.5 \\
construction--barrier--curb & 42.9 & 70.5 & 60.9 \\
construction--barrier--fence & 32.0 & 72.2 & 44.3 \\
construction--barrier--guard-rail & 29.5 & 73.2 & 40.3 \\
construction--barrier--other-barrier & 24.3 & 77.4 & 31.3 \\
construction--barrier--wall & 19.4 & 72.7 & 26.7 \\
construction--flat--bike-lane & 13.0 & 69.9 & 18.7 \\
construction--flat--crosswalk-plain & 32.9 & 75.3 & 43.7 \\
construction--flat--curb-cut & 3.3 & 62.0 & 5.4 \\
construction--flat--parking & 5.9 & 64.2 & 9.2 \\
construction--flat--pedestrian-area & 19.1 & 85.2 & 22.4 \\
construction--flat--rail-track & 11.9 & 70.5 & 16.9 \\
construction--flat--road & 83.1 & 89.1 & 93.3 \\
construction--flat--service-lane & 28.6 & 80.2 & 35.7 \\
construction--flat--sidewalk & 52.4 & 77.6 & 67.6 \\
construction--structure--bridge & 33.1 & 76.6 & 43.2 \\
construction--structure--building & 69.2 & 83.0 & 83.5 \\
construction--structure--tunnel & 8.9 & 56.8 & 15.7 \\
human--person & 54.7 & 78.7 & 69.5 \\
human--rider--bicyclist & 43.3 & 73.6 & 58.8 \\
human--rider--motorcyclist & 38.2 & 70.3 & 54.3 \\
human--rider--other-rider & 7.8 & 52.8 & 14.8 \\
marking--crosswalk-zebra & 46.1 & 76.1 & 60.5 \\
marking--general & 41.1 & 68.6 & 59.9 \\
nature--mountain & 22.1 & 71.8 & 30.8 \\
nature--sand & 4.2 & 81.5 & 5.1 \\
nature--sky & 96.0 & 96.8 & 99.2 \\
nature--snow & 33.8 & 82.3 & 41.1 \\
nature--terrain & 37.8 & 76.9 & 49.2 \\
nature--vegetation & 81.3 & 86.0 & 94.5 \\
nature--water & 17.7 & 75.4 & 23.4 \\
object--banner & 30.6 & 82.3 & 37.1 \\
object--bench & 26.8 & 73.8 & 36.4 \\
object--bike-rack & 6.7 & 71.2 & 9.4 \\
object--billboard & 40.1 & 82.1 & 48.8 \\
object--catch-basin & 35.7 & 75.4 & 47.4 \\
object--cctv-camera & 21.0 & 69.5 & 30.2 \\
object--fire-hydrant & 56.8 & 80.8 & 70.2 \\
object--junction-box & 41.1 & 85.4 & 48.1 \\
object--mailbox & 23.0 & 79.0 & 29.2 \\
object--manhole & 47.7 & 81.2 & 58.8 \\
object--phone-booth & 15.1 & 84.7 & 17.9 \\
object--pothole & 0.6 & 63.0 & 1.0 \\
object--street-light & 46.0 & 74.0 & 62.1 \\
object--support--pole & 33.8 & 70.3 & 48.0 \\
object--support--traffic-sign-frame & 18.8 & 64.4 & 29.2 \\
object--support--utility-pole & 36.9 & 68.4 & 53.9 \\
object--traffic-light & 59.0 & 79.4 & 74.4 \\
object--traffic-sign--back & 39.0 & 74.9 & 52.2 \\
object--traffic-sign--front & 58.8 & 83.8 & 70.2 \\
object--trash-can & 48.5 & 83.7 & 57.9 \\
object--vehicle--bicycle & 37.7 & 72.1 & 52.2 \\
object--vehicle--boat & 17.1 & 67.8 & 25.3 \\
object--vehicle--bus & 54.6 & 87.6 & 62.3 \\
object--vehicle--car & 68.7 & 85.8 & 80.1 \\
object--vehicle--caravan & 0.0 & 0.0 & 0.0 \\
object--vehicle--motorcycle & 45.0 & 73.1 & 61.6 \\
object--vehicle--on-rails & 6.9 & 79.4 & 8.7 \\
object--vehicle--other-vehicle & 22.2 & 74.6 & 29.7 \\
object--vehicle--trailer & 13.6 & 79.3 & 17.1 \\
object--vehicle--truck & 51.6 & 86.3 & 59.8 \\
object--vehicle--wheeled-slow & 27.8 & 70.3 & 39.5 \\
void--car-mount & 51.7 & 85.2 & 60.7 \\
void--ego-vehicle & 71.5 & 90.4 & 79.2 \\ \bottomrule
\end{tabular}
}
\end{table}

\begin{table}[]
\centering
\resizebox{0.3\textwidth}{!}{%
\begin{tabular}{@{}lccc@{}}
\toprule
\textbf{Class} & \textbf{PQ} & \textbf{SQ} & \textbf{RQ} \\ \midrule
road & 97.7 & 98.0 & 99.7 \\
sidewalk & 75.3 & 83.8 & 89.9 \\
building & 87.8 & 89.4 & 98.2 \\
wall & 25.5 & 71.2 & 35.8 \\
fence & 27.0 & 71.5 & 37.7 \\
pole & 48.3 & 64.6 & 74.8 \\
traffic-light & 44.7 & 68.6 & 65.2 \\
traffic-sign & 66.1 & 75.9 & 87.0 \\
vegetation & 88.6 & 90.3 & 98.2 \\
terrain & 28.9 & 73.4 & 39.3 \\
sky & 86.2 & 92.3 & 93.4 \\
person & 51.6 & 76.9 & 67.0 \\
rider & 53.5 & 71.7 & 74.6 \\
car & 64.8 & 83.2 & 77.8 \\
truck & 53.3 & 86.3 & 61.7 \\
bus & 72.9 & 88.5 & 82.4 \\
train & 65.6 & 83.1 & 78.9 \\
motorcycle & 44.5 & 72.3 & 61.5 \\
bicycle & 42.2 & 71.6 & 58.9 \\ \bottomrule
\end{tabular}
}
\end{table}
